# Supplementary material for: Clustering Categorical Time Series into Unknown Number of Clusters: A Perfect Simulation based Approach
Source: arXiv:1311.2422 source file (2013-11-11)
Supplement: Supplementary file 1 [file appendix.tex]

\section{Proof that the full conditional densities of $\gamma_{st}$ are log-concave}
\label{sec:log_concave}

For the sake of convenience we re-arrange the factors of the full conditional
of $\gamma_{s^*t^*}$ as follows:
\begin{align}
[\gamma_{\ell,s^*t^*}\mid Z,C,\bgamma_{-s^*,-t^*},k]&\propto 
\prod_{\ell=1}^k\frac{\Gamma\left(\sum_{i:z_i=j}\sum_{j:c_j=\ell}N_{i,s^*t^*}+\gamma_{s^*t^*}\right)}
{\Gamma\left(\gamma_{s^*t^*}\right)}\notag\\
&\times 
\left(\frac{\Gamma\left(\sum_{t=1}^K\gamma_{s^*t}\right)}
{\Gamma\left(\sum_{t=1}^K\sum_{i:z_i=j}\sum_{j:c_j=\ell}N_{i,s^*t}+\sum_{t=1}^K\gamma_{s^*t}\right)}\notag\\
&\times \gamma^{a_{jk}-1}_{s^*t^*}\exp\left(-b_{jk}\gamma_{s^*t^*}\right)
\label{eq:fullcond_gamma2}
\end{align}

\section{Proof that ${F^L}_i$ and ${F^U}_i$ are distribution functions}
\label{sec:distribution_function}

Letting $X_{-i}$ denote all unknown variables other than $z_i$
we need to show that for almost all $X_{-i}$ the following holds:
\begin{itemize}
\item[(i)] $\lim_{h\rightarrow -\infty}F^L_i(h)=\lim_{h\rightarrow -\infty}F^U_i(h)=0$.
\item[(ii)] $\lim_{h\rightarrow \infty}F^L_i(h)=\lim_{h\rightarrow \infty}F^U_i(h)=1$.
\item[(iii)] For any $x_1\geq x_2$, $F^L_i(x_1)\geq F^L_i(x_2)$ and $F^U_i(x_1)\geq F^U_i(x_2)$.
\item[(iv)] $\lim_{h\rightarrow x+}F^L_i(h)=F^L_i(x)$ and $\lim_{h\rightarrow x+}F^U_i(h)=F^U_i(x)$.
\end{itemize}

{\bf Proof:} 
Let $X_{-i}$ denote all unknown variables other than $z_i$. To prove (i), note that for all $h<1$, 
$F_i(h\mid X_{-i})=0$ for almost all $X_{-i}$. Hence, by (\ref{eq:full_cond_z}) of MB
and by definition,
both $F^L_i(h)$ and $F^U_i(h)$ are 0 with probability 1. Hence, $\lim_{h\rightarrow -\infty}F^L_i(h)=\lim_{h\rightarrow -\infty}F^U_i(h)=0$
almost surely.

To prove (ii) note that for all $h>p$, $F_i(h\mid X_{-i})=1$ for almost all $X_{-i}$. Hence, for $h>p$, $F^L_i(h)=F^U_i(h)=1$,
that is, $\lim_{h\rightarrow \infty}F^L_i(h)=\lim_{h\rightarrow \infty}F^U_i(h)=1$ for almost all $X_{-i}$.

To show (iii), let $h_1>h_2$. Then, since $F_i(\cdot\mid X_{-i})$ is a distribution function satisfying monotonicity, it holds that 
$F^L_i(h_2)=\inf_{X_{-i}}F_i(h_2\mid X_{-i})\leq F_i(h_2\mid X_{-i})\leq F_i(h_1\mid X_{-i})$ for almost all $X_{-i}$.
Hence, $F^L_i(h_2)\leq \inf_{X_{-i}}F_i(h_1\mid X_{-i})=F^L_i(h_1)$. 
Similarly, $F^U_i(h_1)=\sup_{X_{-i}}F_i(h_1\mid X_{-i})\geq F_i(h_1\mid X_{-i})\geq F_i(h_2\mid X_{-i})$ for almost all $X_{-i}$. Hence, 
$F^U_i(h_1)\geq\sup_{X_{-i}}F_i(h_2\mid X_{-i})=F^U_i(h_2)$.

To prove (iv), first observe that due to the monotonicity property (iii), the following hold for any $x$:
\begin{eqnarray}
\lim_{h\rightarrow x+}F^L_i(h)&\geq& F^L_i(x)\label{eq:mono1}\\
\lim_{h\rightarrow x+}F^U_i(h)&\geq& F^U_i(x)\label{eq:mono2}
\end{eqnarray}
Then observe that, due to discreteness, $F_i(\cdot\mid X_{-i})$ is constant in the interval $[x,x+\delta)$ for some $\delta>0$.
Since the supports of $F^L_i$, $F^U_i$ and $F_i(\cdot\mid X_{-i})$ for almost all $X_{-i}$ are same, $F^L_i$ and $F^U_i$
must also be constants in $[x,x+\delta)$. This implies that equality holds in (\ref{eq:mono1}) and (\ref{eq:mono2}).

Hence, both $F^L_i$ and $F^U_i$ satisfy all the properties of distribution functions.
\\[2mm]
{\bf Remark:} The right continuity property formalized by (iv) not be true for continuous variables.
Suppose $X\sim U(0, \theta)$, $\theta>0$. Here the distribution function is
$F(x\mid \theta) = \frac{x}{\theta}$, $0<x<\theta<\infty$. But
\[
\lim_{x\rightarrow 0+} \sup_{\theta}\frac{x}{\theta}\nonumber\\
= \lim_{x\rightarrow 0+} 1\nonumber\\
= 1\nonumber\\
\]
and,
\[
\sup_{\theta} \lim_{x\rightarrow 0+} \frac{x}{\theta}\nonumber\\
= \sup_{\theta} 0\nonumber\\
= 0\nonumber\\
\]
As a consequence of the above problem, attempts to construct suitable stochastic bounds for the 
continuous parameters $(\Pi_p,\Theta_p)$ may not be fruitful. In our case such problem does not arise
since we only need to construct bounds for the discrete random variables to achieve our goal.

\section{Proof of validity of our CFTP algorithm}
\label{sec:validity}

%Let us suppose that the individual chains are started from
%all possible states of Z. The individual chains are updated in following Gibbs sampling sequence $\Theta$, Z. Denote
%the chain of Z at time t started from j-th started at time n as 
%$X_{n}^{t, j}$.

{\bf Theorem:} The terminal chains coalesce almost surely in finite time and the value obtained at 
time $t=0$ is a a realization from the target distribution. 
\\[2mm]
{\bf Proof:}

%We have to prove the following
%three facts:\\

%1. The algorithm will finish in finite time and produce a value; say it $X_0$.\\

%2. For each j, $D(X_{n}^{t, j}) \rightarrow \pi$ as t$\rightarrow -\infty$. \\

%3. For each j, $X_0^{t, j} \rightarrow X_0$ as t$\rightarrow -\infty$.\\

%{\bf Proof:} 
%{\it Fact 1:} Here at each step the terminal chains at time t depends only on R(t), the uniform random variable used for updating at
%time t. 

Let $z^L_{it}$ denote the realization obtained at time $t$ by inverting 
$F^U_i$, that is, $z^L_{it}={F^U_i}^{-}(R_{z_i,t})$, where 
$\{R_{z_i,t}; i=1,\ldots,n;t=1,2,\ldots\}$ is a common set of $U(0,1)$ random numbers
which are $iid$ with respect to both $i$ and $t$.
used to simulate
$Z=(z_1,\ldots,z_n)'$ at time $t$ for Markov chains starting at all possible initial values.
Similarly, let $z^U_{it}={F^L_i}^{-}(R_{z_i,t})$. 
Clearly, for any $z_{it}=F^{-}_i(R_{z_i,t}\mid X_{-i})$ started with any initial value and for any 
$X_{-i}$, $z^L_{it}\leq z_{it}\leq z^U_{it}$ for all $i$ and $t$.

For $i=1,\ldots,n$ and for $j=1,2,\ldots$, we denote by $S^j_i$ the event
\[ z^L_{i,-2^j}(-2^{j-1})=z^U_{i,-2^j}(-2^{j-1}), \] which signifies that
the terminal chains and hence the individual chains started at
$t=-2^j$ will coalesce at $t=-2^{j-1}$. 
It is important to note that both $F^L_i$ and $F^U_i$ are irreducible
which has the consequence that the probability of $S^j_i$, $P(S^j_i)>\epsilon_i>0$,
for some positive $\epsilon_i$. Since, for fixed $i$, $\{S^j_i;j=1,2,\ldots\}$ depends only upon the random numbers
$\{R_{z_i,t};t= -2^j,\ldots,-2^{j-1}\}$, $\{S^j_i;j=1,2,\ldots\}$ are independent with respect to $j$. Moreover, for fixed $j$, $S^j_i$  
depends only upon the $iid$ random numbers $\{R_{z_i,-2^j};i=1,\ldots,n\}$. Hence, $\{S^j_i;i=1,\ldots,n;j=1,2,\ldots\}$ are 
independent with respect to both $i$ and $j$.

Let $\epsilon=\min\{\epsilon_1,\ldots,\epsilon_n\}$. Then 
due to independence of $\{S^j_i;i=1,\ldots,n\}$, it follows that for $j=1,2,\ldots$,
$\bar S^j=\cap_{i=1}^nS^j_i$ are independent, and
\begin{equation}
P\left(\bar S^j\right)\geq \epsilon^n
\label{eq:indep1}
\end{equation}
The rest of the proof resembles the proof of Theorem 2 of \ctn{Casella01}. In other words,
\begin{eqnarray}
P(\mbox{No coalescence after T iterations} )&\leq & \prod_{j=1}^T\left\{1-P(\bar S^j)\right\}\label{eq:indep2}\\
&=& \left\{(1-\epsilon^n)\right\}^T\rightarrow 0\ \ \mbox{as} \ \ T\rightarrow\infty\label{eq:indep3}.
\end{eqnarray}
Thus, the probability of coalescence is 1. That the time to coalesce is almost surely finite follows
from the Borel-Cantelli lemma, exactly as in \ctn{Casella01}. 

The realization obtained at time $t=0$ after occurrence of the coalescence 
event $\bar S_j$ for some $j$ yields $Z=Z_0$ exactly from its marginal posterior
distribution. Given this $Z_0$, drawing $\Pi_{p0}$ from the full conditional distribution
(\ref{eq:full_cond_pi}) of MB 
and then drawing $\Theta_{p0}$ sequentially from (\ref{eq:full_cond_lambda}) 
and (\ref{eq:full_cond_mu}) of MB 
given $Z_0$ and $\Pi_{p0}$, yields a realization $(Z_0,\Pi_{p0},\Theta_{p0})$ exactly from
the target posterior. The proof of this exactness follows readily from the general proof (see, for example,
\ctn{Prop96}, \ctn{Casella01})
that if convergent Markov chains colasece in a CFTP algorithm during time $t\leq 0$, then the realization obtained 
at time $t=0$ is exactly from the stationary distribution.

%\subsubsection{Note:}
%\label{subsubsec:note}
%We have to notice whether $K_i=0$ and $P_i=1$ for every time t, that
%is maximum and minimum over $x_{-i}$ is 1 and 0 respectively or the
%maxima/minima does not exist. In that case we may eliminate
%those $x_{-i}$ from the whole space for which values 0 and 1 are
%attained. If those points are limit points of the space then we can
%reduce our space into the one does not have those limit points.
%One easy solution may be to make compact set for the parameter
%space and maximize or minimize subject to that probability of attaining any value  does not become zero or the upper and lower chain has at least one point in common for which probability is non-null
%for both the chains. \\

%Under the above assumption, we have $P(S_i)=c >\epsilon >0$. Also
%$S_i$'s are independent, i=$1, 2, \ldots,$. Easy to show that
%\[ \sum_{i=1}^{\infty} P(S_i)\hspace{2mm}=\hspace{2mm}\infty
%\implies P(S_i\hspace{2mm}infinitely\hspace{2mm}often) = 1\],
%from Borel-Cantelli Lemma.

%So, almost surely the terminal chains and hence the individual chains would coalesce.

%{\it Fact 2.} Note that $\mathcal{D}(X_0^{t,j})$ = $\mathcal{D}(X_t^{0,j})$ because they are
%both the distribution of a Markov chain that starts in state j and
%progresses through t time steps. $\mathcal{D}(X_t^{0,j})\rightarrow \pi$ is the stationary distribution.

%{\it Fact 3.} Fact 1 tells that all chains coalesces almost surely before time 0. Call the time of coalescence as N.
%Then for all t$<$N, $X_0^{t,j}$ = $X_0$, which implies Fact 3. 

\section{Uniform ergodicity}
\label{sec:uniform_ergodicity}

Let $P(\cdot,\cdot)$ denote a Markov transition kernel where 
$P(x,A)$ denotes transition from the state $x$ to the set $A\in\mathcal B$, $\mathcal B$
being the associated Borel $\sigma$-algebra.
If we can show that for all $x$ in the state space the following minorization holds:
\[ P(x, A)\geq\epsilon Q(A),\hspace{2mm}A\in {\mathcal{B}}, \]
for some $0<\epsilon\leq 1$ and for some probability measure $Q(\cdot)$,
then $P(\cdot,\cdot)$ is uniformly ergodic. 

In our mixture model situation the Gibbs sampling transition kernel is
\begin{eqnarray}
&&\left[Z^{(t)},\Pi^{(t)}_p,\Theta^{(t)}_p\mid Z^{(t-1)},\Pi^{(t-1)}_p,\Theta^{(t-1)}_p\right]\nonumber\\
&& \ \ = \left[Z^{(t)}\mid\Pi^{(t-1)}_p,\Theta^{(t-1)}_p,Y\right]\left[\Pi^{(t)}_p\mid Z^{(t)},Y\right]\left[\Theta^{(t)}_p\mid Z^{(t)},\Pi^{(t)}_p,Y\right]\nonumber\\
&& \ \ \geq \left\{\inf_{\Pi^{(t-1)}_p,\Theta^{(t-1)}_p}\left[Z^{(t)}\mid\Pi^{(t-1)}_p,\Theta^{(t-1)}_p,Y\right]\right\}
\left[\Pi^{(t)}_p\mid Z^{(t)},Y\right]\left[\Theta^{(t)}_p\mid Z^{(t)},\Pi^{(t)}_p,Y\right]
\label{eq:minorization}
\end{eqnarray}
The infimum in inequality (\ref{eq:minorization}) is finite since both $\Pi^{(t-1)}_p$ and $\Theta^{(t-1)}_p$ are bounded.

Denoting the right hand side of inequality (\ref{eq:minorization}) by
$g(Z^{(t)},\Pi^{(t)}_p,\Theta^{(t)}_p)$, we put 
\begin{equation}
\epsilon = \sum_{Z} \int_{\Pi_p}\int_{\Theta_p} g(Z,\Pi_p,\Theta_p)d\Pi_pd\Theta_p>0. 
\label{eq:epsilon}
\end{equation}
Since $g(\cdot)$ is bounded above by the Gibbs transition kernel which integrates to 1, it follows
from (\ref{eq:epsilon}) that $0<\epsilon\leq 1$. 
Hence, identifying the density of the $Q$-measure as $g(\cdot)/ \epsilon$, the minorization
condition required for establishment of uniform ergodicity of our Gibbs sampling chain is seen to hold.

\section{Proof that coalescence of $C$ implies the coalescence of $S$}
\label{sec:s_coalescence}

Let $C=(c_1,\ldots,c_M)'$ be coalescent.
For convenience of illustration assume that after simulating each $c_j$, followed by drawing $\theta_j$ depending
upon the simulated value of $c_j$, the entire set $S$ is obtained from the updated set of parameters $\Theta_M$.
Note that in practice, only $s_j$ will be obtained immediately after updating $c_j$ and $\theta_j$. Let $S_{-j}=\{s_1,\ldots,s_{j-1},s_{j+1},\ldots,s_M\}$.
Then $c_{j+1}=\ell$ denotes the $\ell$-th distinct element of $S_{-j}$. If $\{1,\ldots,d_j\}$ are the distinct components in $S_{-j}$,
$d_j$ being the number of distinct components, and $\ell\leq s_j$, then $s_{j+1}=\ell$. On the other hand, if $\ell<c_{j+1}\leq d_j+1$, then $s_{j+1}=s_j+1$.

Now note that $s_1=1$, which is always coalescent. If $c_2>1$, then $s_2=2$, else $s_2=1$, for all Markov chains. Hence, $s_2$
is coalescent. If $c_3>s_2$, then $s_3=s_2+1$, else $s_3=c_3$. Since $s_2$ is coalescent,
then so is $s_3$. In general, if $c_{j+1}>s_j$, then $s_{j+1}=s_j+1$, else $s_{j+1}=c_{j+1}$. Since $s_1,\ldots,s_j$ are coalescent, hence
so is $s_{j+1}$, for $j=1,\ldots,M-1$. In other words, $S$ must coalesce if $C$ coalesces.
